# Supplementary material for: MR-GDINO: Efficient Open-World Continual Object Detection
Source: arXiv:2412.15979 source file (2024-12-23)
Supplement: Supplementary file 1 [file supp.tex]

\section{Parameter Analysis}\label{sec:supp_params}

\section{More Analysis}\label{sec:supp_more_analysis}

\section{More Visualization Results}\label{sec:supp_more_vis}

\section{Limitation}\label{sec:supp_limitation}
The limitation of our work is two-fold. Firstly, our retrieval module is still a heuristic method, which may not fully exploit the potential anti-forgetting abilities and restrict the detection performance. Secondly, whether the memory and retrieval mechanisms can further improve the open-world detection results or not is still unexplored, which is left for further investigation. 

\section{Broader Impact}
{\method} is based on a large-scale pretrained open-world object detector~\cite{liu2023grounding}, and only fine-tunes a few learnable parameters to ensure promising detection performance on old, new, and unseen categories under few-shot continual adaptation scenarios. Compared to previous continual open-world object detectors, {\method} largely mitigates catastrophic forgetting on unseen categories and performs better on seen categories with few-shot fine-tuning data, which is more practical for real-world applications. However, {\method} is still fully data-driven, and should be cautious with potential negative impact from biased data.
